# Supplementary material for: Design and Control of a Midair-Reconfigurable Quadcopter using Unactuated Hinges
Source: arXiv:2103.16632 source file (2021-12-17)
Supplement: Supplementary file 1 [file appendix.tex]

\appendix[Thrust limits derivation]

Here we derive the limits placed on the relevant control variables such that the arms of the vehicle do fold during flight as described in Section \ref{sec:thrustLimits}.
